# Supplementary material for: A comparative study of immersed boundary method and interpolated bounce-back scheme for no-slip boundary treatment in the lattice Boltzmann method: Part I, laminar flows
Source: arXiv:1906.05445 source file (2019-06-13)
Supplement: Supplementary file 1 [file Appendix.tex]

\section{Appendix: LBGK equation with a forcing term}
In this Appendix, we prove the semi-implicit forcing scheme of Cheng \& Li and the fully explicit forcing scheme of Guo are actually identical with different definition.
The BGK Boltzmann equation on a set of discrete velocity $\vec{e}_{\alpha}$ reads
\begin{equation}
    \frac{\partial f_{\alpha}}{\partial t} + \vec{e}_{\alpha}\cdot \frac{\partial f_{\alpha}}{\partial \vec{x}} + \vec{a}\cdot\frac{\partial f_{\alpha}}{\partial \vec{e}_{\alpha}} = -\frac{1}{\tau}\left[f_{\alpha}-f_{\alpha}^{(eq)}\right].
    \label{eq:BoltzmannBGK}
\end{equation}
Integrate Eq.~(\ref{eq:BoltzmannBGK}) along the characteristic line and apply the trapezoid rule to the collision term and the forcing term, one obtains
\begin{equation}
\begin{split}
  &f_{\alpha}\left(\vec{x}+\vec{e}_{\alpha}\delta t,t+\delta t\right) - f_{\alpha}\left(\vec{x},t\right) = \\
  &-\frac{\delta t}{2\tau}\left[f_{\alpha}^{(n+1)}-f_{\alpha}^{(eq)(n+1)}\right]-\frac{\delta t}{2\tau}\left[f_{\alpha}^{(n)}-f_{\alpha}^{(eq)(n)}\right]-\frac{\delta t}{2}F_{\alpha}^{(n+1)} - \frac{\delta t}{2}F_{\alpha}^{(n)},
  \end{split}
    \label{eq:integralLBGK}
\end{equation}
where the superscripts $(n+1)$ and $(n)$ are the shorthand notation for the terms at future time $t+\delta t$ and the current time $t$, respectively. $F_{\alpha}^{(n)} = \vec{a}^{(n)}\cdot \frac{\partial f_{\alpha}^{(n)}}{\partial \vec{e}_{\alpha}}$, $F_{\alpha}^{(n+1)} = \vec{a}^{(n+1)}\cdot \frac{\partial f_{\alpha}^{(n+1)}}{\partial \vec{e}_{\alpha}}$.

The LBGK equation using Guo's scheme is fully explicit. In order to derive Guo's forcing scheme, define
\begin{equation}
\begin{split}
   &\bar{f_{\alpha}}\left(\vec{x}+\vec{e}_{\alpha}\delta t,t+\delta t\right)  = f_{\alpha}\left(\vec{x}+\vec{e}_{\alpha}\delta t,t+\delta t\right)+\frac{\delta t}{2\tau}\left[f_{\alpha}^{(n+1)}-f_{\alpha}^{(eq)(n+1)}\right]+\frac{\delta t}{2}F_{\alpha}^{(n+1)},\\
   &\bar{f_{\alpha}}\left(\vec{x},t\right)  = f_{\alpha}\left(\vec{x},t\right)+\frac{\delta t}{2\tau}\left[f_{\alpha}^{(n)}-f_{\alpha}^{(eq)(n)}\right]+\frac{\delta t}{2}F_{\alpha}^{(n)},
   \end{split}
    \label{eq:guoredefinition}
\end{equation}
to fully absorb the implicit terms, Eq.~(\ref{eq:integralLBGK}) becomes
\begin{equation}
     \bar{f_{\alpha}}\left(\vec{x}+\vec{e}_{\alpha}\delta t,t+\delta t\right) - \bar{f_{\alpha}}\left(\vec{x},t\right) = \frac{\delta t}{\bar{\tau}}\left[\bar{f_{\alpha}}\left(x,t\right)-\bar{f}_{\alpha}^{(eq)}\left(x,t\right)\right]-\left(1-\frac{1}{2\bar{\tau} }\right)F_{\alpha}\left(x,t\right)\delta t,
    \label{eq:LBGK1}
\end{equation}
where $\bar{f}_{\alpha}^{(eq)}\left(x,t\right) = f_{\alpha}^{(eq)}\left(x,t\right)$, $\bar{\tau} = \tau + 0.5 = \nu/c_s^2 + 0.5$.

By definition, 
\begin{equation}
\begin{split}
F_{\alpha} &= \vec{a}\cdot \frac{\partial f_{\alpha}}{\partial \vec{e}_{\alpha}}\approx \vec{a}\cdot \frac{\partial f_{\alpha}^{(eq)}}{\partial \vec{e}_{\alpha}}=-\vec{a}\cdot \frac{\left(\vec{e}_{\alpha}-\vec{u}\right)}{c_s^2}f_{\alpha}^{(eq)} \\
&= -\frac{\vec{F}}{\rho}\cdot \frac{\left(\vec{e}_{\alpha}-\vec{u}\right)}{c_s^2}\rho w_{\alpha}\left[1+\frac{\left(\vec{e}_{\alpha}\cdot \vec{u}\right)}{c_s^2}+\frac{\left(\vec{e}_{\alpha}\cdot \vec{u}\right)^2}{2c_s^4}-\frac{\left(\vec{u}\cdot \vec{u}\right)}{2c_s^2}\right].
\end{split}
    \label{eq:mesoscopicforcing}
\end{equation}
Note that the approximation in Eq.~(\ref{eq:mesoscopicforcing}) is allowed since to reproduce the N-S equations, only the Chapman-Enskog expansion to the order of $\tau$, {\it i.e.}, 
\begin{equation}
    f_{\alpha} = f_{\alpha}^{(eq)} - \tau\left[\frac{\partial f^{(eq)}}{\partial t} + \vec{e}_{\alpha}\cdot \frac{\partial f^{(eq)}}{\partial \vec{x}}\right] + O\left(\tau^2\right),
    \label{eq:firstorderCE}
\end{equation}
is required, while the leading order truncation error of approximating $\vec{F}\cdot \frac{\partial f_{\alpha}}{\partial \vec{e}_{\alpha}}$ with $\vec{F}\cdot \frac{\partial f_{\alpha}^{(eq)}}{\partial \vec{e}_{\alpha}}$ is on the order of $O\left(\tau^2\right)$. The last part of Eq.~(\ref{eq:mesoscopicforcing}) can be further simplified by eliminate all the terms on the order of $O(Ma^3)$ or higher, with the notice that $\|\vec{F}\|\sim \|\vec{u}\|/\delta t\sim O\left(Ma\right)$, as
\begin{equation}
    F_{\alpha} = -\vec{F}\cdot  w_{\alpha}\left[\frac{\left(\vec{e}_{\alpha}-\vec{u}\right)}{c_s^2}+\frac{\left(\vec{e}_{\alpha}\cdot \vec{u}\right)\vec{e}_{\alpha}}{c_s^4}\right].
    \label{eq:guoforcingscheme}
\end{equation}
Apparently, substituting Eq.~(\ref{eq:guoforcingscheme}) into Eq.~(\ref{eq:mesoscopicforcing}), the resulting last term is precisely the mesoscopic forcing term in Guo's formulation. When Eq.~(\ref{eq:mesoscopicforcing}) is used, the forcing term should be calculated with the boundary force at the currently time, rather than the future time $t+\delta t$ as the distribution function has been redefined to absorb all the implicity. 

On the other hand, when Cheng \& Li's scheme is used, the LBGK equation has a semi-implicit forcing term. To derive its formula, define
\begin{equation}
\begin{split}
   &\tilde{f_{\alpha}}\left(\vec{x}+\vec{e}_{\alpha}\delta t,t+\delta t\right)  = f_{\alpha}\left(\vec{x}+\vec{e}_{\alpha}\delta t,t+\delta t\right)+\frac{\delta t}{2\tau}\left[f_{\alpha}^{(n+1)}-f_{\alpha}^{(eq)(n+1)}\right],\\
   &\tilde{f_{\alpha}}\left(\vec{x},t\right)  = f_{\alpha}\left(\vec{x},t\right)+\frac{\delta t}{2\tau}\left[f_{\alpha}^{(n)}-f_{\alpha}^{(eq)(n)}\right],
   \end{split}
    \label{eq:chengredefinition}
\end{equation}
Eq.~(\ref{eq:integralLBGK}) becomes
\begin{equation}
     \tilde{f_{\alpha}}\left(\vec{x}+\vec{e}_{\alpha}\delta t,t+\delta t\right) - \tilde{f_{\alpha}}\left(\vec{x},t\right) = \frac{\delta t}{\bar{\tau}}\left[\tilde{f_{\alpha}}\left(x,t\right)-\tilde{f}_{\alpha}^{(eq)}\left(x,t\right)\right]-\frac{F_{\alpha}'^{(n+1)}\delta t}{2}-\frac{F_{\alpha}'^{(n)}\delta t}{2},
    \label{eq:LBGK2}
\end{equation}
where the form of $F_{\alpha}'^{(n)}$ and $F_{\alpha}'^{(n+1)}$ are derived in Eq.~(\ref{eq:guoforcingscheme}). An iteration process~\cite{cheng2007,zhang2016} is usually required to determine $F_{\alpha}'^{(n+1)}$, since it is a function of future velocity $\vec{u}\left(t+\delta t\right)$. A simple replacement of $F_{\alpha}'^{(n+1)} = F_{\alpha}'\left(\vec{x}+\vec{e}\delta t,t+\delta t\right)$ with $F_{\alpha}'^{(n+1)} = F_{\alpha}'\left(\vec{x}+\vec{e}_{\alpha}\delta t,t\right)$ or $F_{\alpha}'^{(n+1)} = F_{\alpha}'\left(\vec{x},t\right)$(as did by Kang \& Hassan in their Eq.~(20c)) is questionable.
